# Supplementary material for: On the unimportance of memory for the time non-local components of the Kadanoff-Baym equations
Source: arXiv:2306.06225 source file (2023-09-04)
Supplement: Supplementary file 1 [file SM.pdf]

# Supplementary information for "On the unimportance of memory for the time non-local components of the Kadanoff-Baym equations"

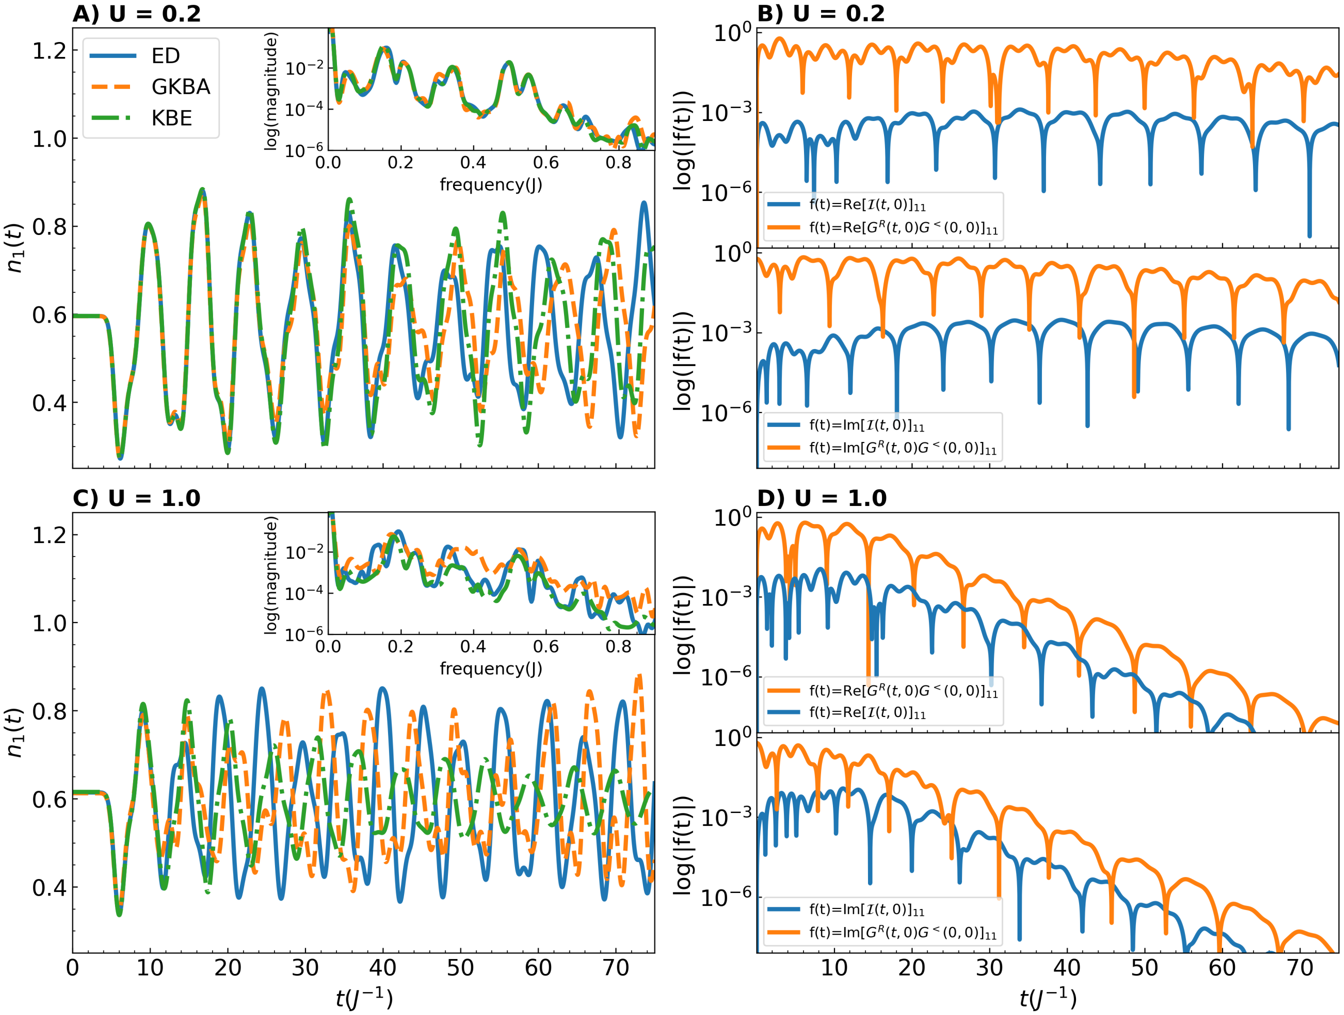


FIG. S1: Comparison between HF-GKBA, KBE and exact dynamics in a 4-site model with exponentially decaying long-range hopping and a long wavelength excitation. The magnitude of the excitation is $E = 0.5J$. Panels A and C show a comparison of the time-dependent density on the first site of a 4-site chain for $U = 0.2J$ and $U = 1.0J$ respectively. Panels B and D show the magnitudes of the integral and non-integral terms in equation (15) in the main text along the time trajectory $[0, t]$ in the same systems. Inset: Frequency spectrum for the trajectories shown plotted on a semi-log scale.

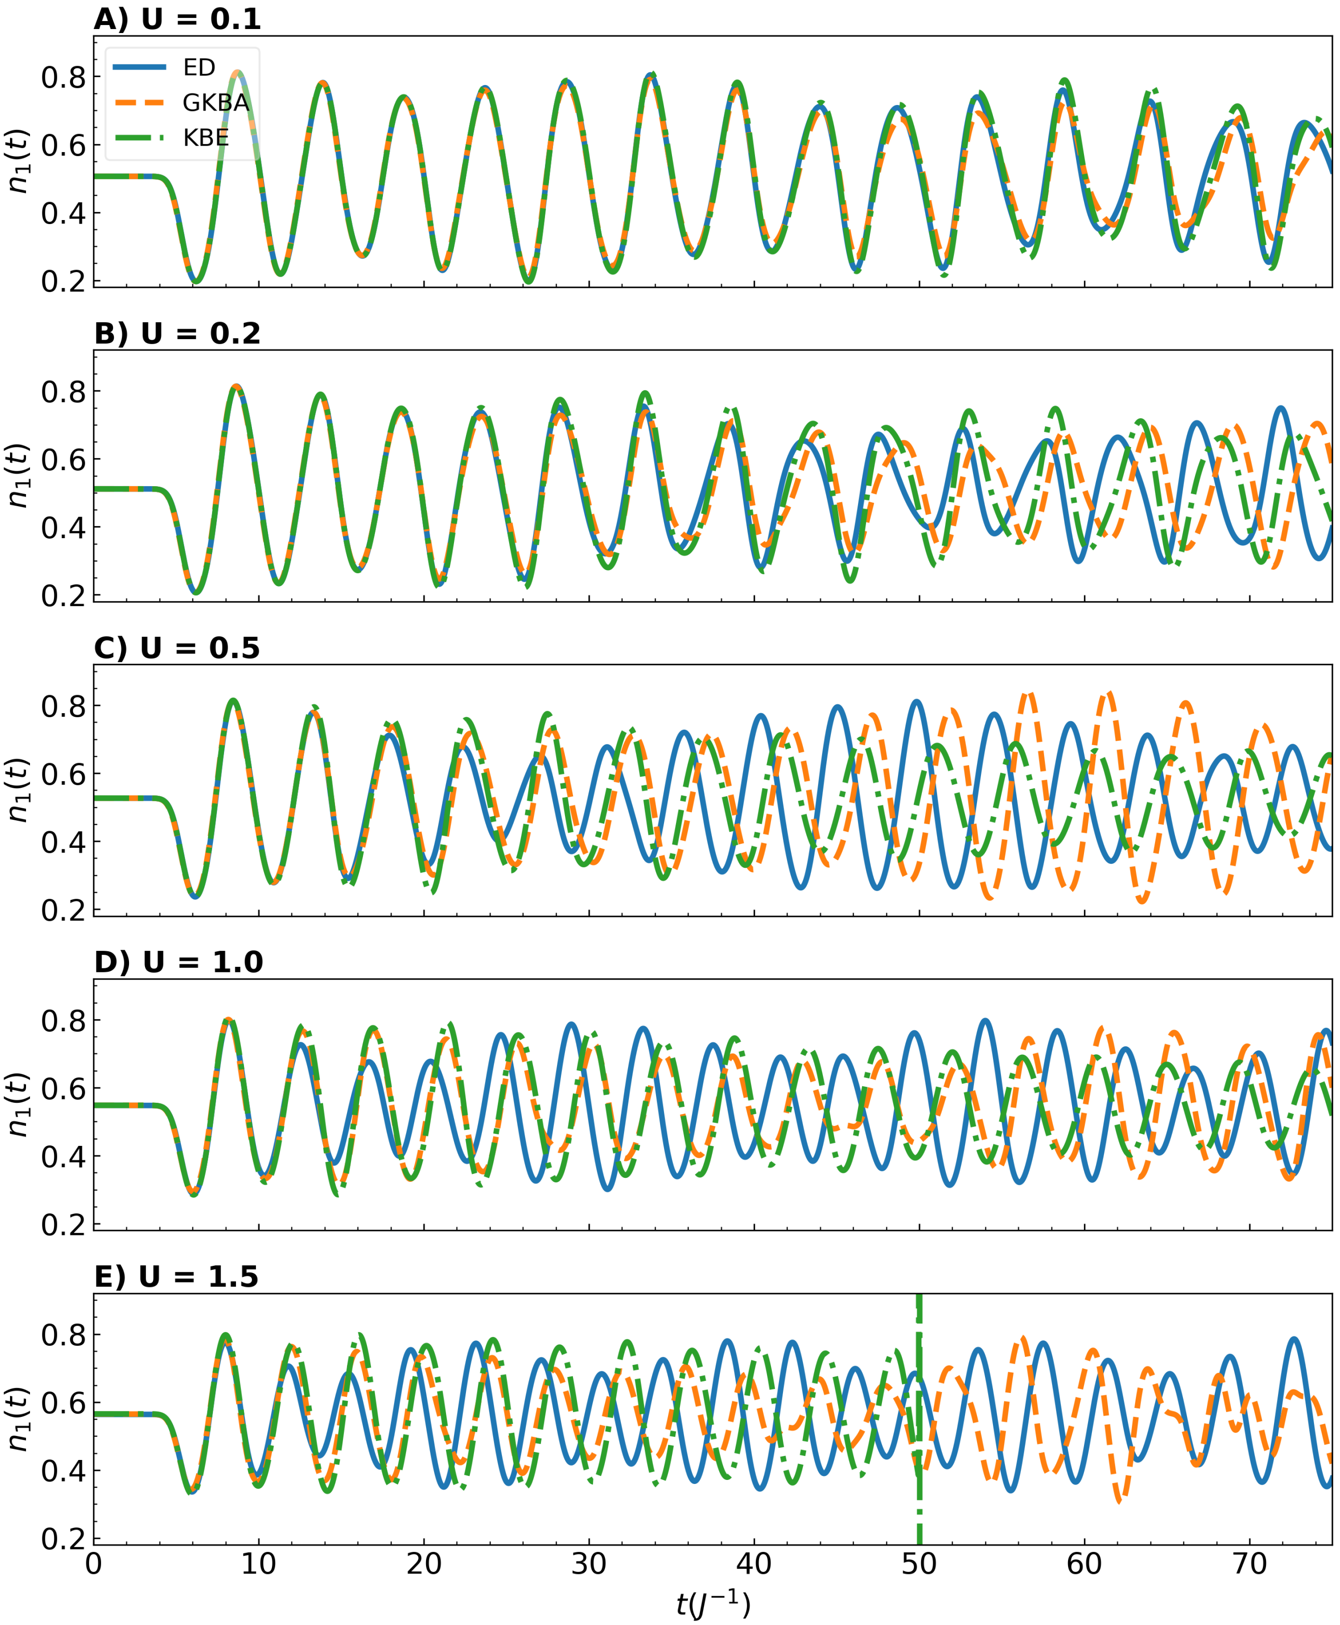


FIG. S2: Time-dependent density of the first site for the model described in section IV A in the main text with nearest neighbor hopping. The system is excited with the long wavelength limit pulse with magnitude $E = 0.5J$. Panels A-E show different strengths of the interaction parameter.

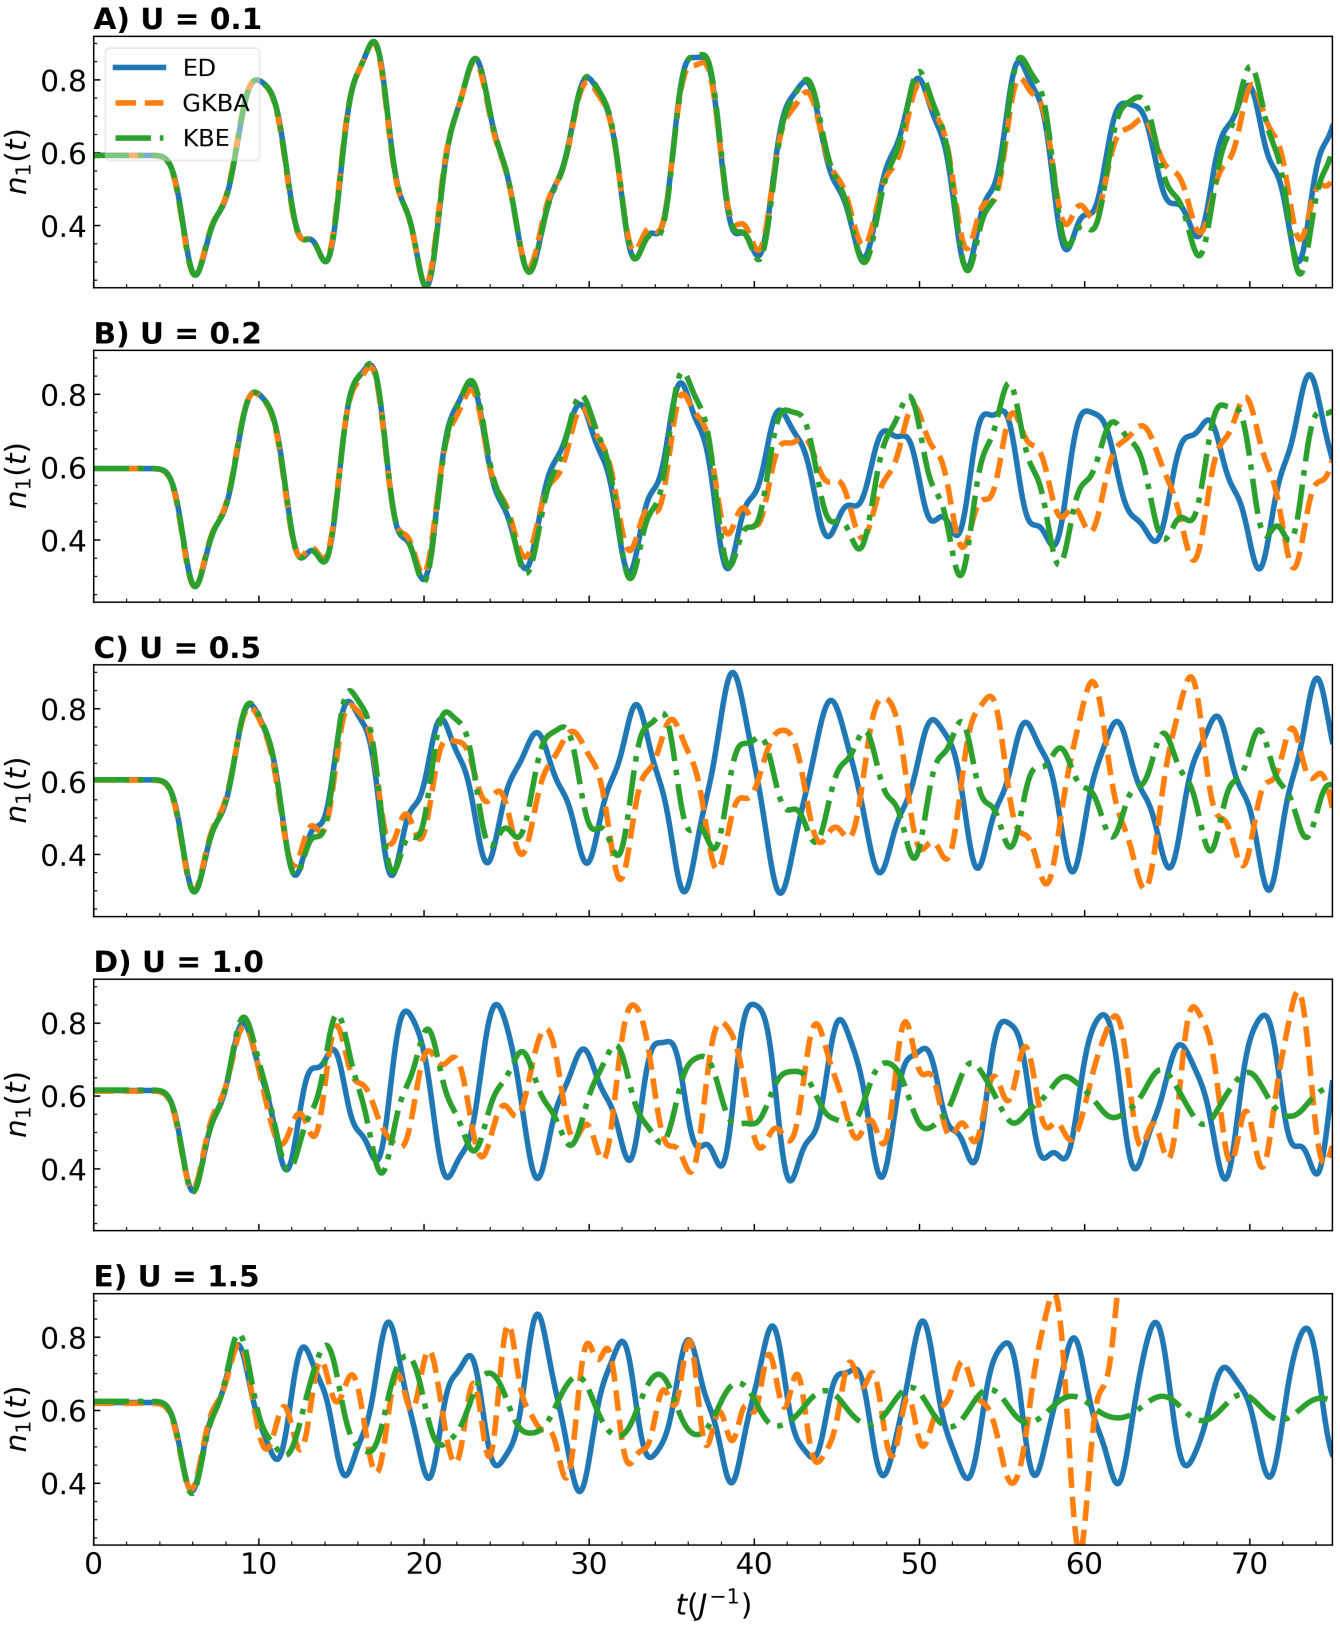


FIG. S3: Time-dependent density of the first site for the model described in section IV A in the main text with long range hopping. The system is excited with the long wavelength limit pulse with magnitude $E = 0.5J$. Panels A-E show different strengths of the interaction parameter.

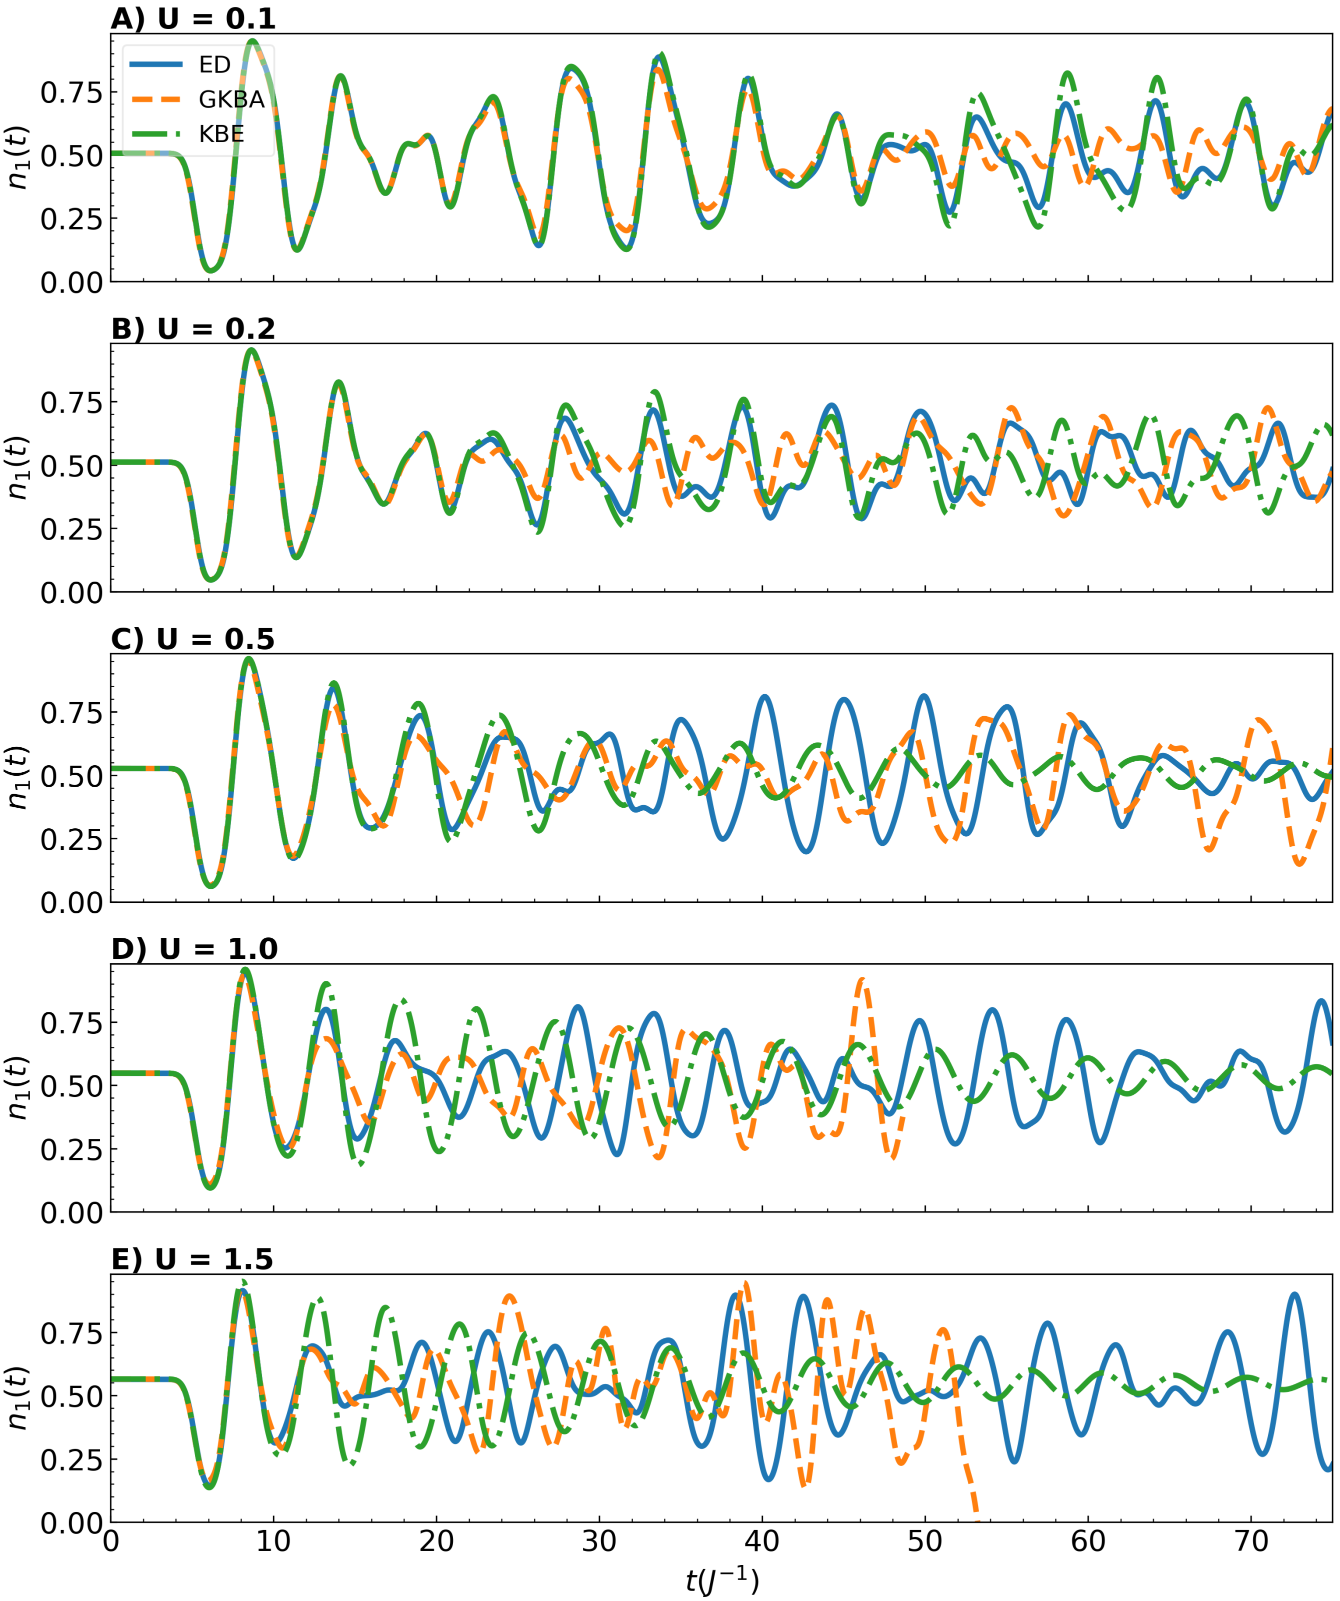


FIG. S4: Time-dependent density of the first site for the model described in section IV A in the main text with nearest neighbor hopping. The system is excited with the long wavelength limit pulse with magnitude $E = 1.0J$. Panels A-E show different strengths of the interaction parameter.

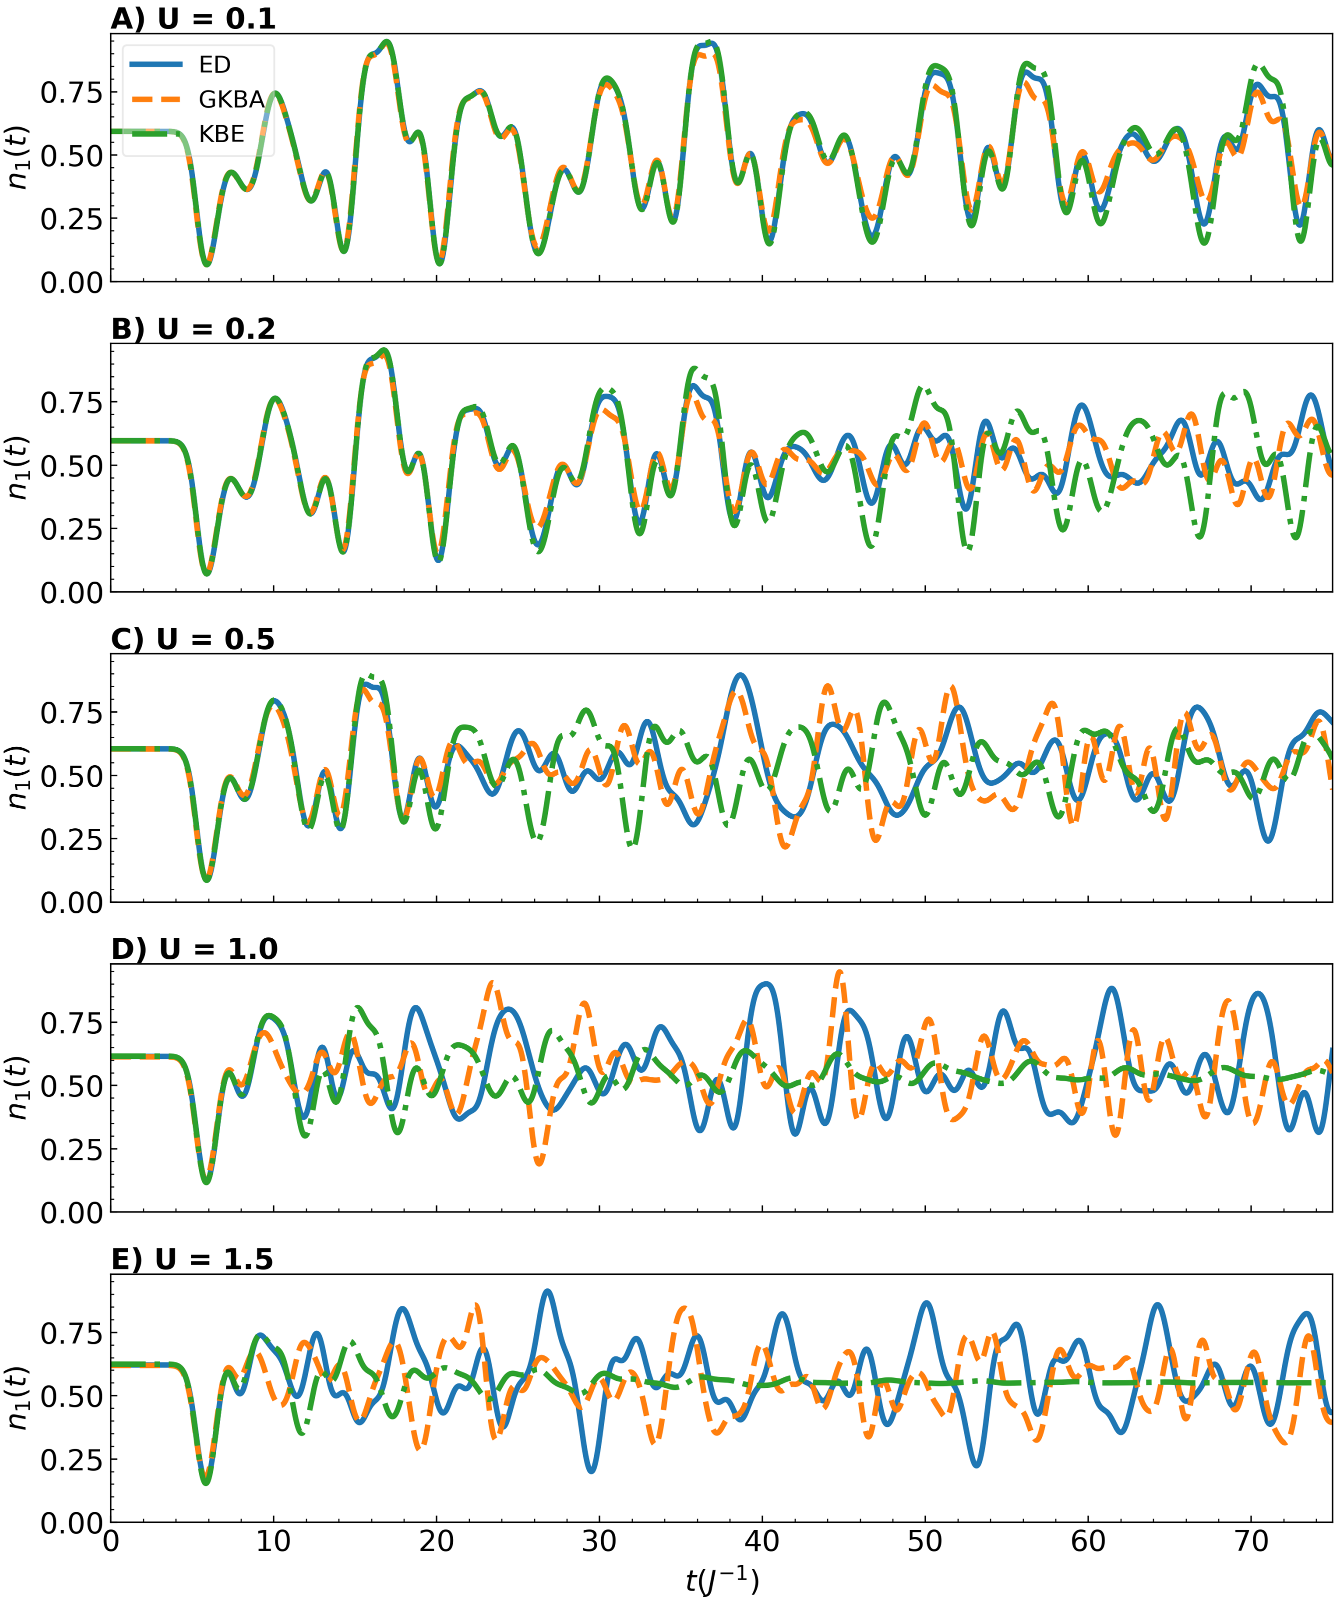


FIG. S5: Time-dependent density of the first site for the model described in section IV A in the main text with long range hopping. The system is excited with the long wavelength limit pulse with magnitude $E = 1.0J$. Panels A-E show different strengths of the interaction parameter.

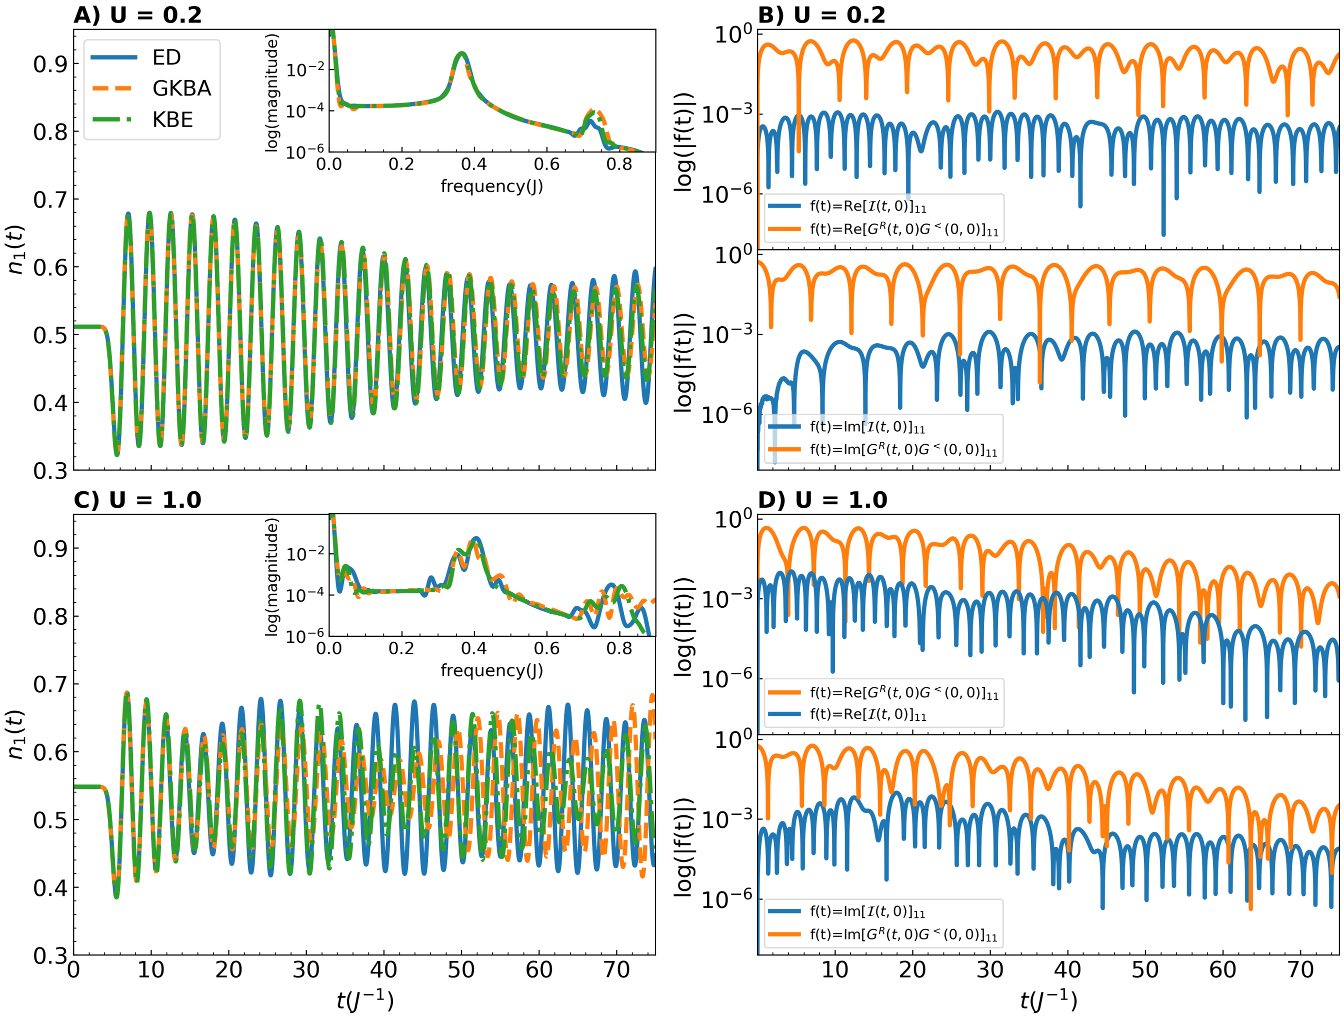


FIG. S6: Comparison between HF-GKBA, KBE and exact dynamics in a 4-site model with nearest neighbor hopping and a short wavelength excitation. The magnitude of the excitation is $E = 0.5J$. Panels A and C show a comparison of the time-dependent density on the first site of a 4-site chain for $U = 0.2J$ and $U = 1.0J$ respectively. Panels B and D show the magnitudes of the integral and non-integral terms in equation (15) in the main text along the time trajectory $[0, t]$ in the same systems. Inset: Frequency spectrum for the trajectories shown plotted on a semi-log scale.

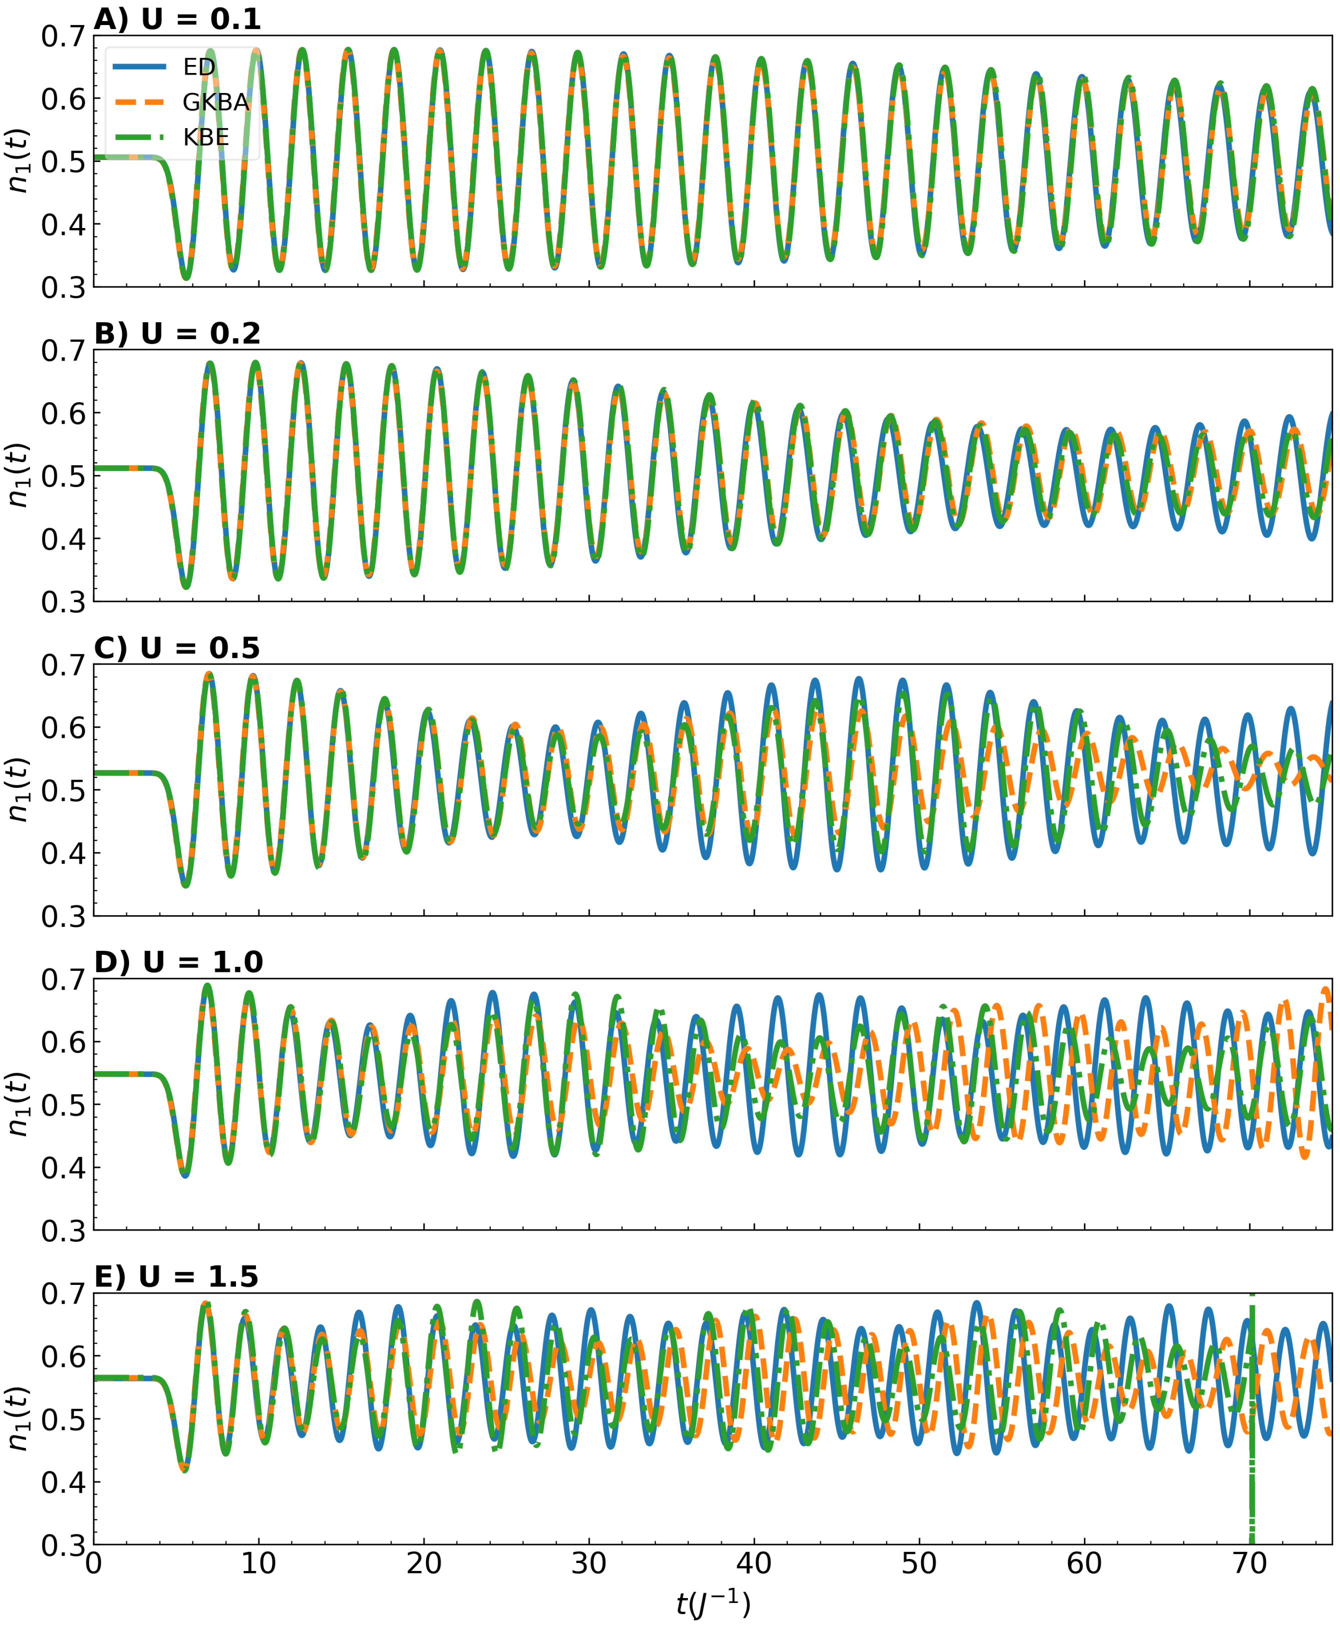


FIG. S7: Time-dependent density of the first site for the model described in section IV A in the main text with nearest neighbor hopping. The system is excited with the short wavelength limit pulse with magnitude $E = 0.5J$. Panels A-E show different strengths of the interaction parameter.

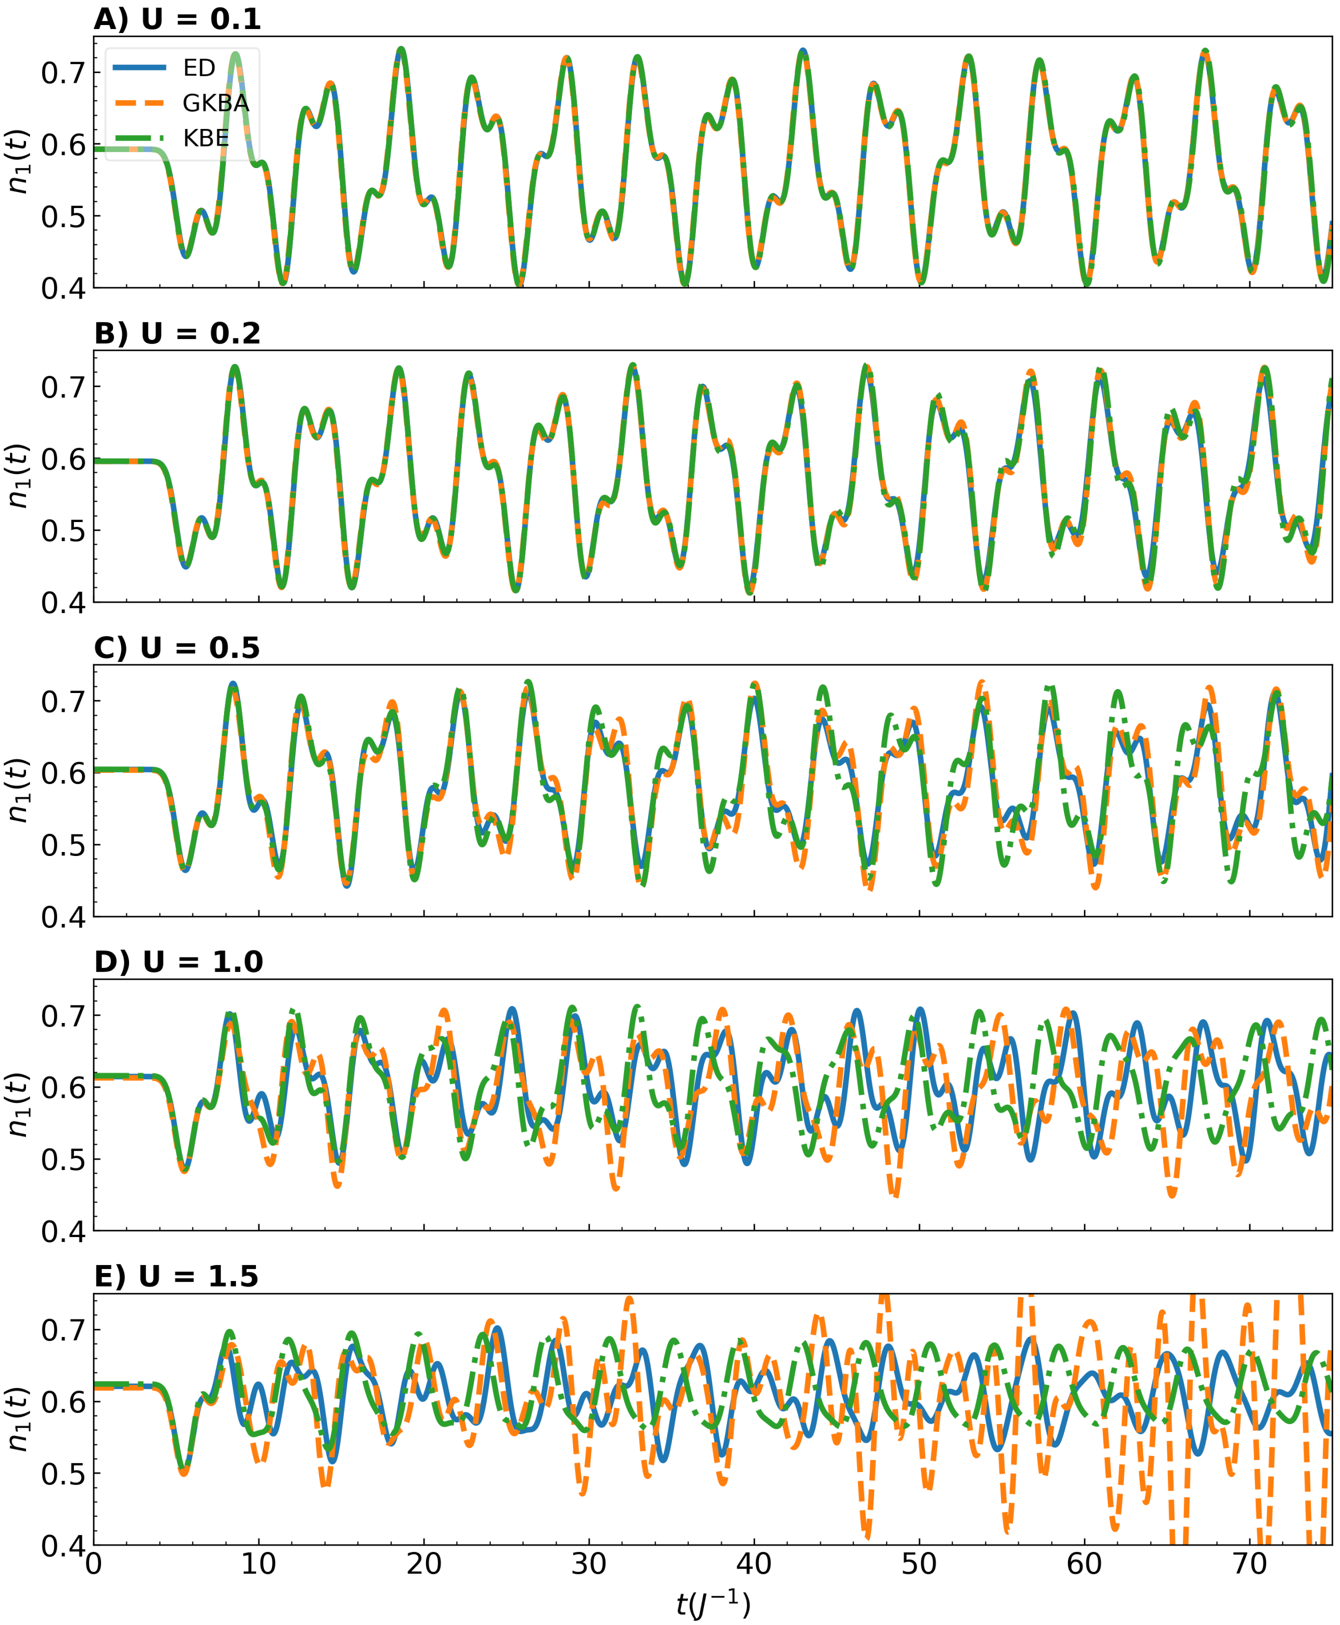


FIG. S8: Time-dependent density of the first site for the model described in section IV A in the main text with long range hopping. The system is excited with the short wavelength limit pulse with magnitude $E = 0.5J$. Panels A-E show different strengths of the interaction parameter.

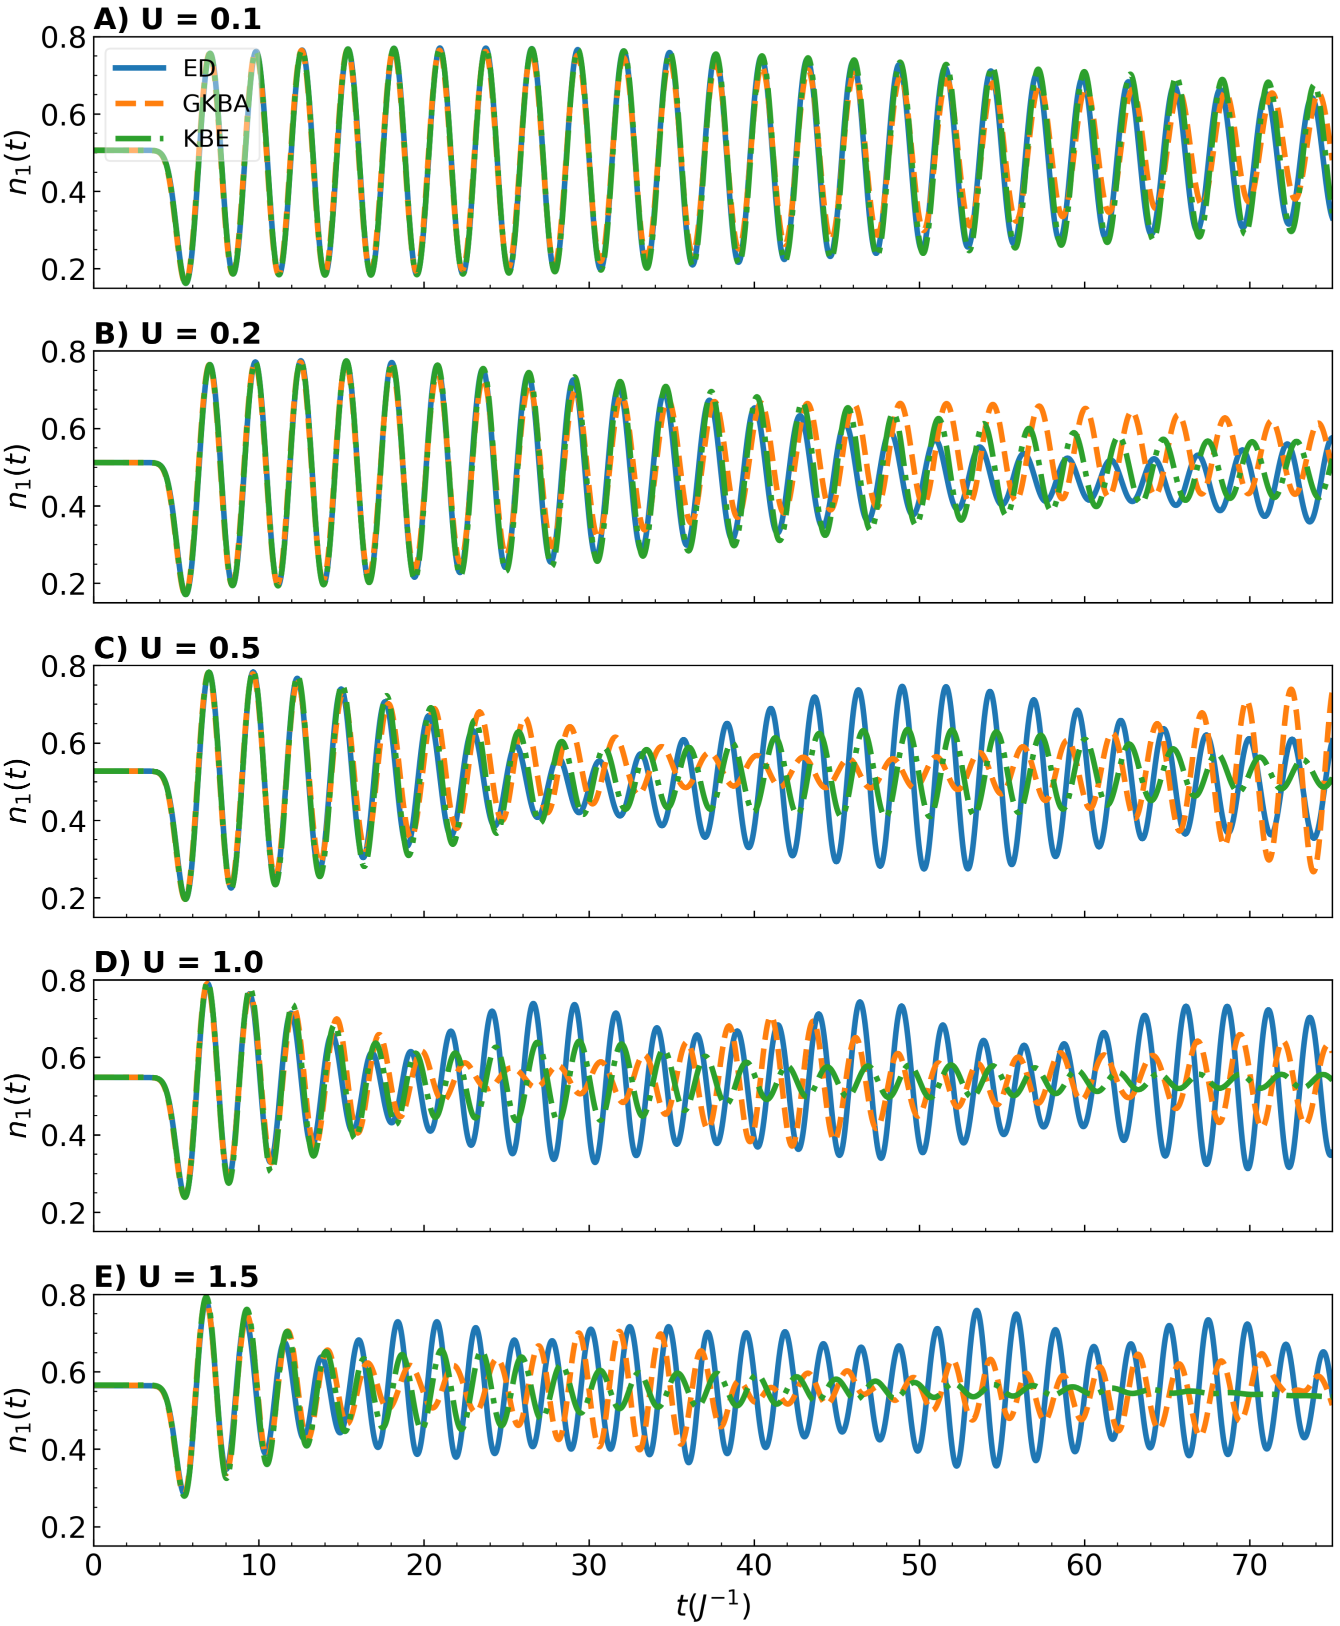


FIG. S9: Time-dependent density of the first site for the model described in section IV A in the main text with nearest neighbor hopping. The system is excited with the short wavelength limit pulse with magnitude $E = 1.0J$. Panels A-E show different strengths of the interaction parameter.

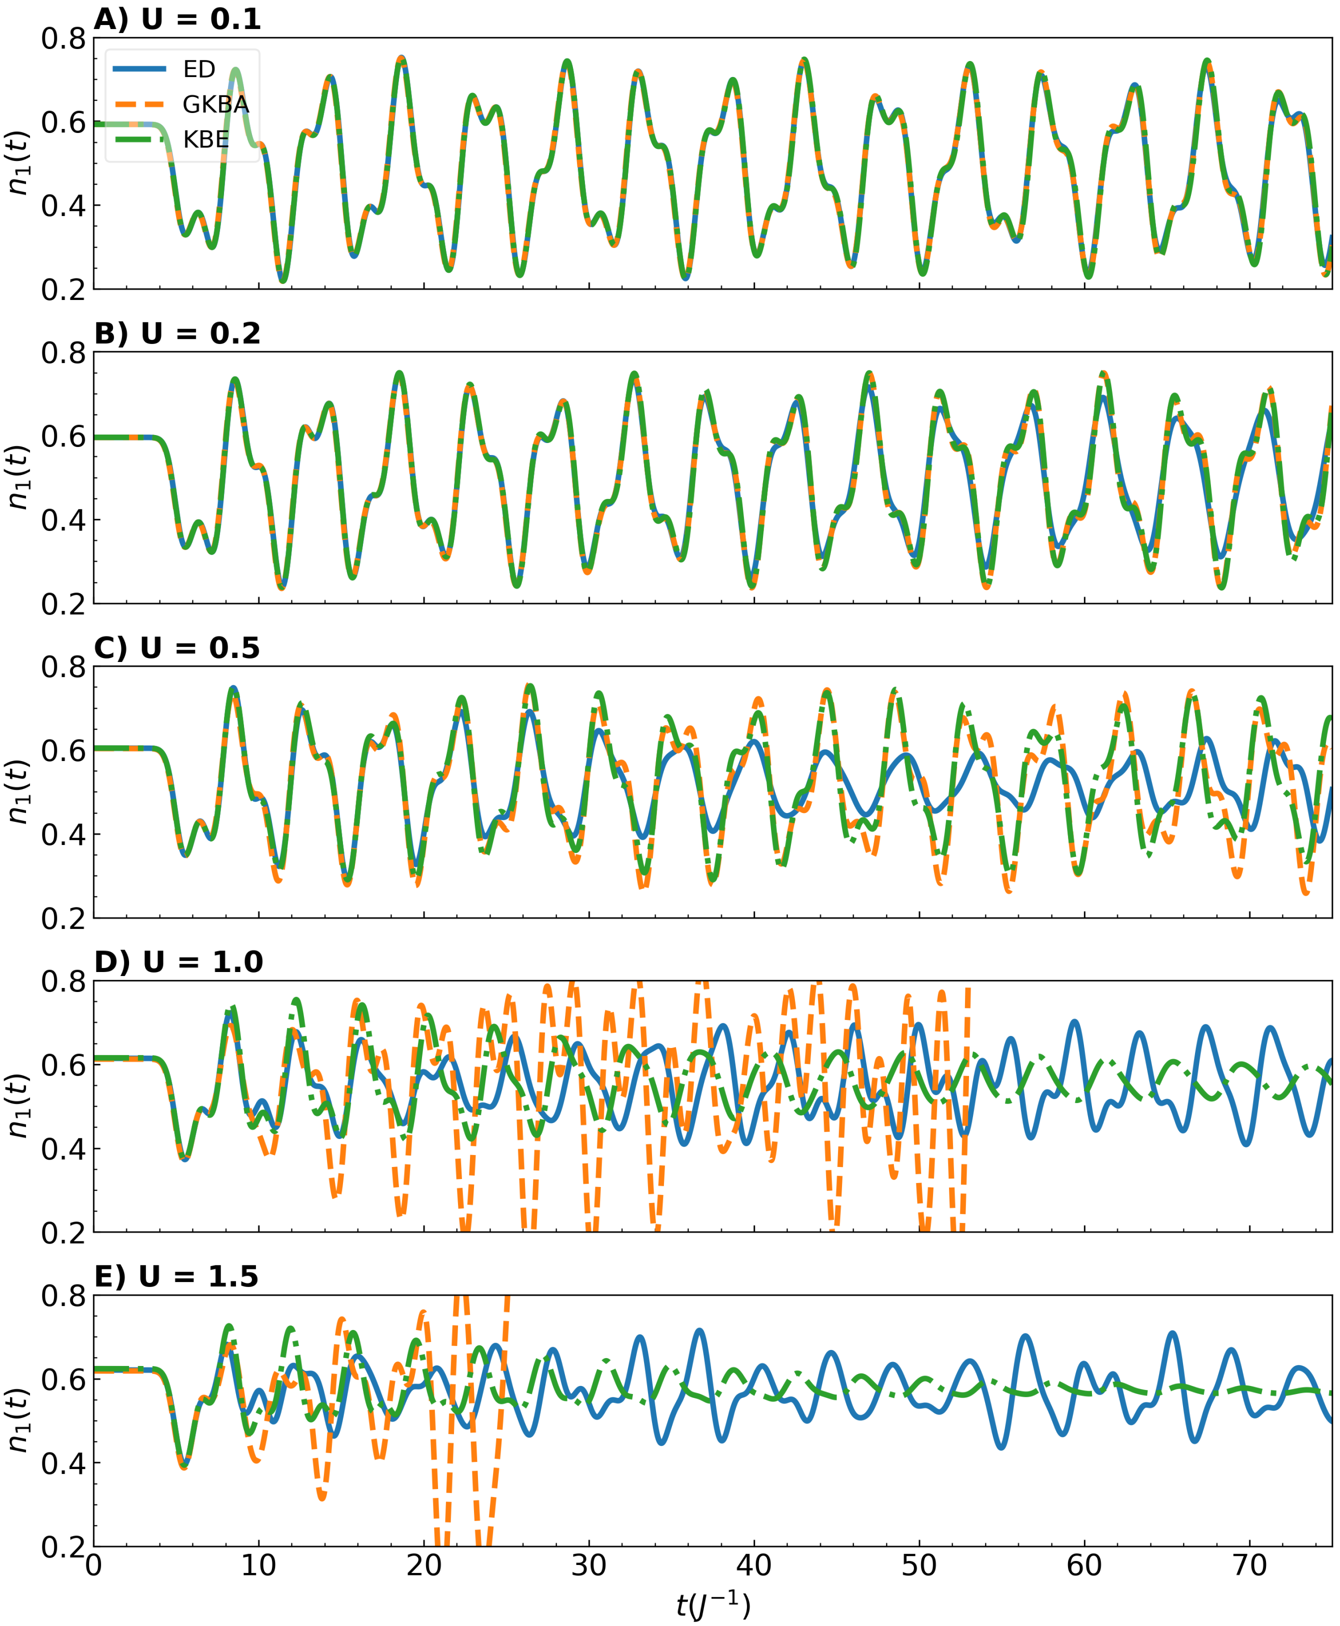


FIG. S10: Time-dependent density of the first site for the model described in section IV A in the main text with long range hopping. The system is excited with the short wavelength limit pulse with magnitude $E = 1.0J$. Panels A-E show different strengths of the interaction parameter.

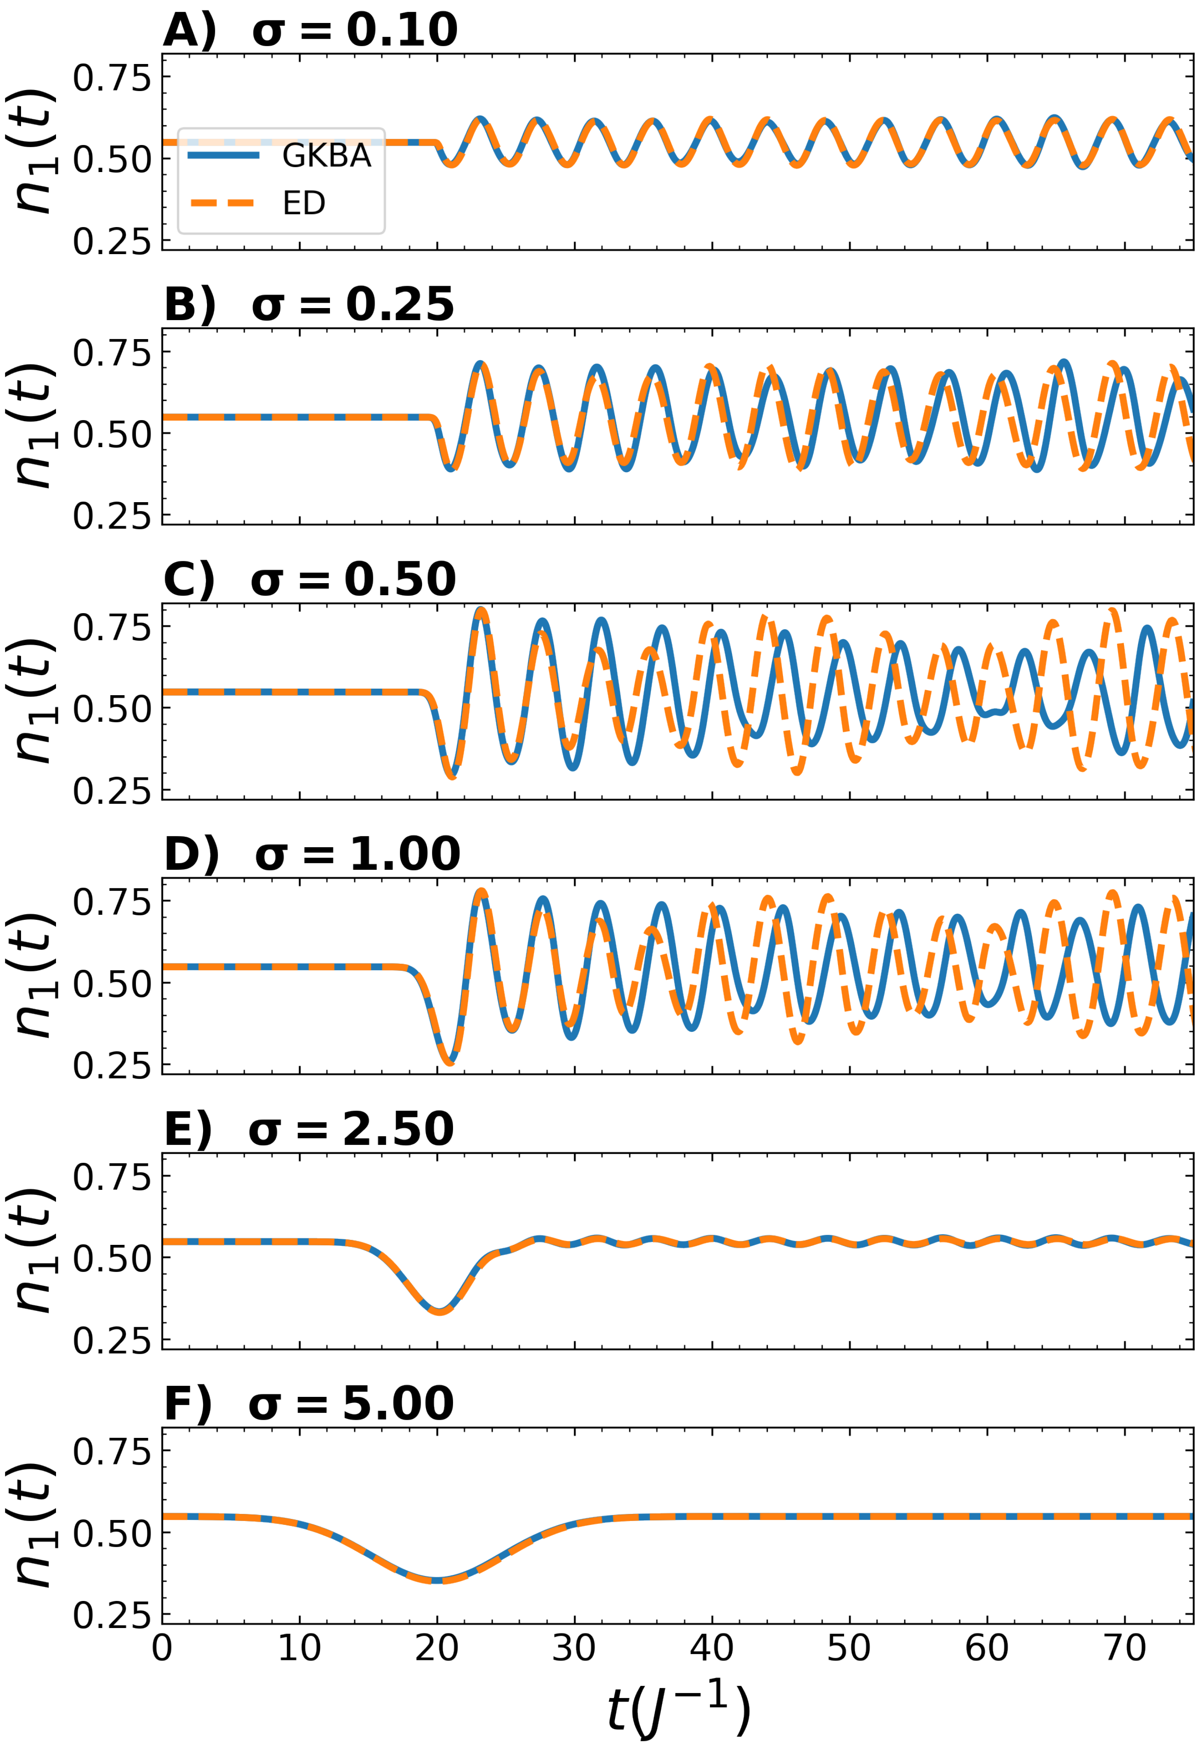


FIG. S11: Time-dependent density of the first site for the model described in section IV A in the main text with nearest neighbor hopping. The system is excited with the long wavelength limit pulse with magnitude $E = 0.5J$. Panels A-F show different values of the pulse width parameter $\sigma$.

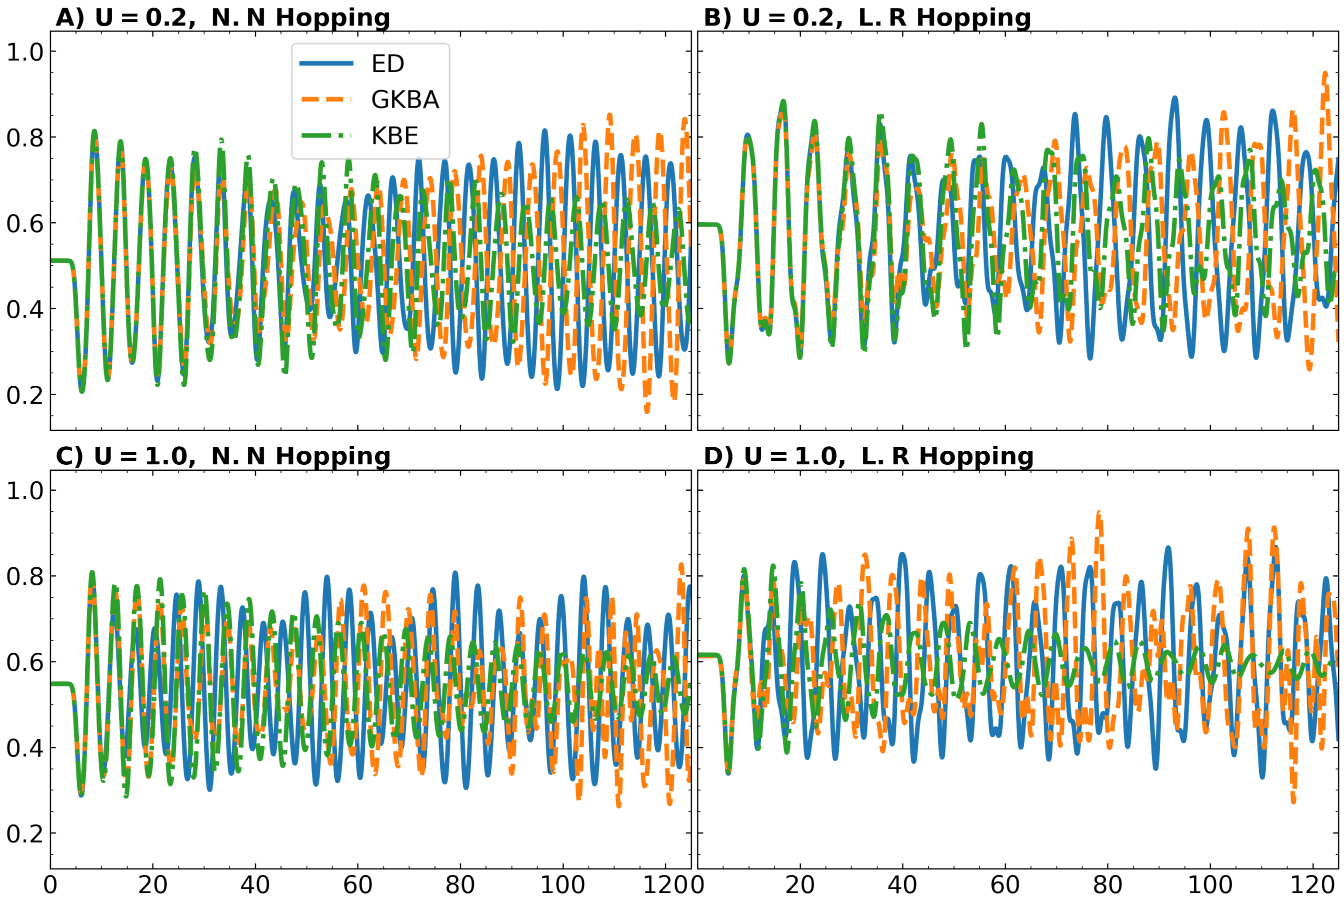


FIG. S12: Time-dependent density of the first site for the models described in section IVA(long range hopping and nearest neighbor hopping) with 4 sites after being excited with the long wavelength limit pulse with magnitude $E = 0.5J$. Different panels show different combinations of type of hopping and interaction strengths.

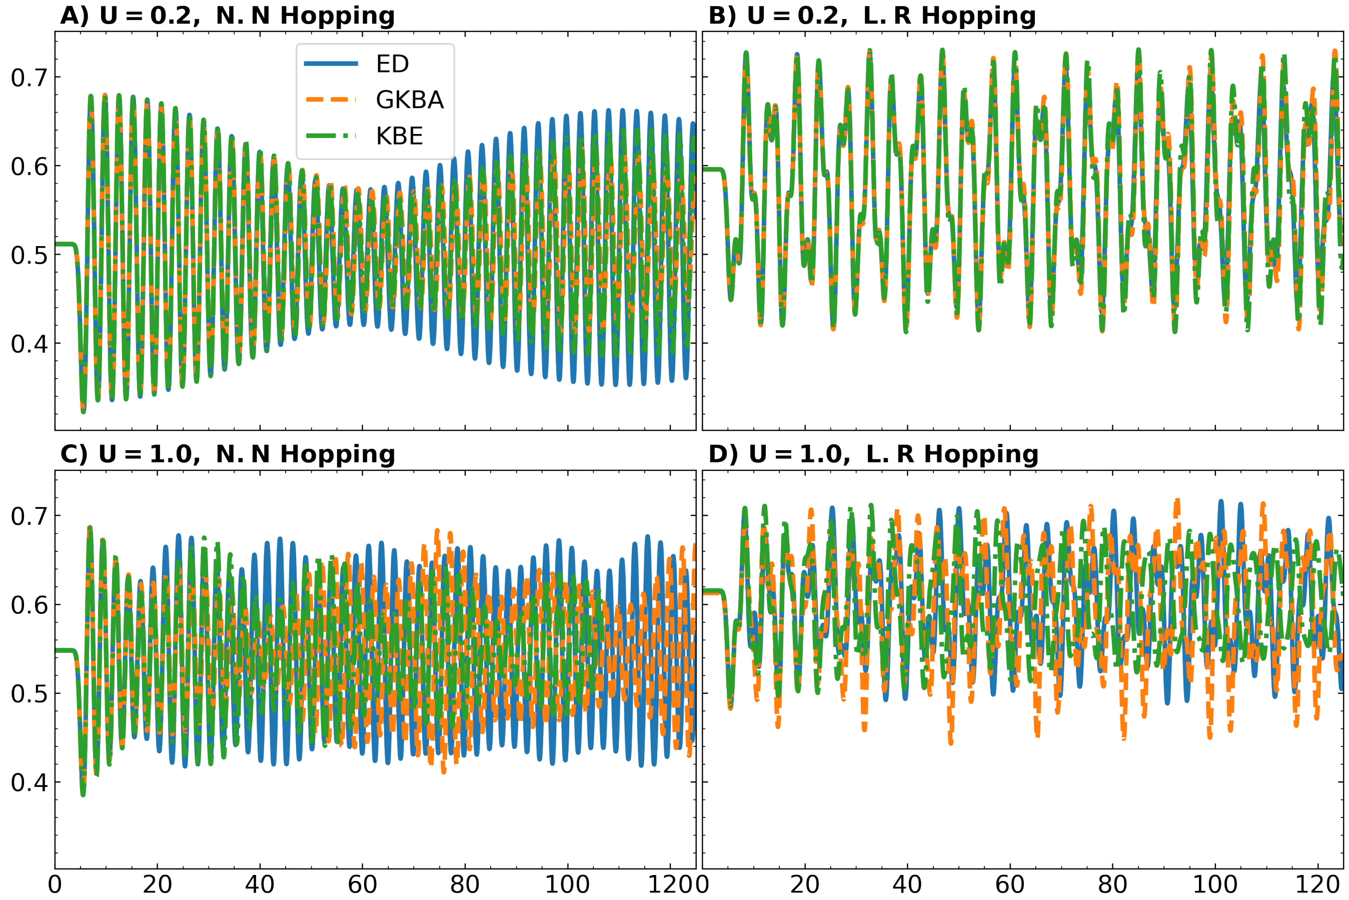


FIG. S13: Time-dependent density of the first site for the models described in section IVA(long range hopping and nearest neighbor hopping) with 4 sites after being excited with the short wavelength limit pulse with magnitude $E = 0.5J$. Different panels show different combinations of type of hopping and interaction strengths.
